# Supplementary material for: FLAG: Flow-based 3D Avatar Generation from Sparse Observations
Source: arXiv:2203.05789 source file (2022-03-11)
Supplement: Supplementary file 1 [file supp_results.tex]

\begin{figure*}[!ht]
    \centering
    \begin{tabular}{c}
         \includegraphics[width=\textwidth]{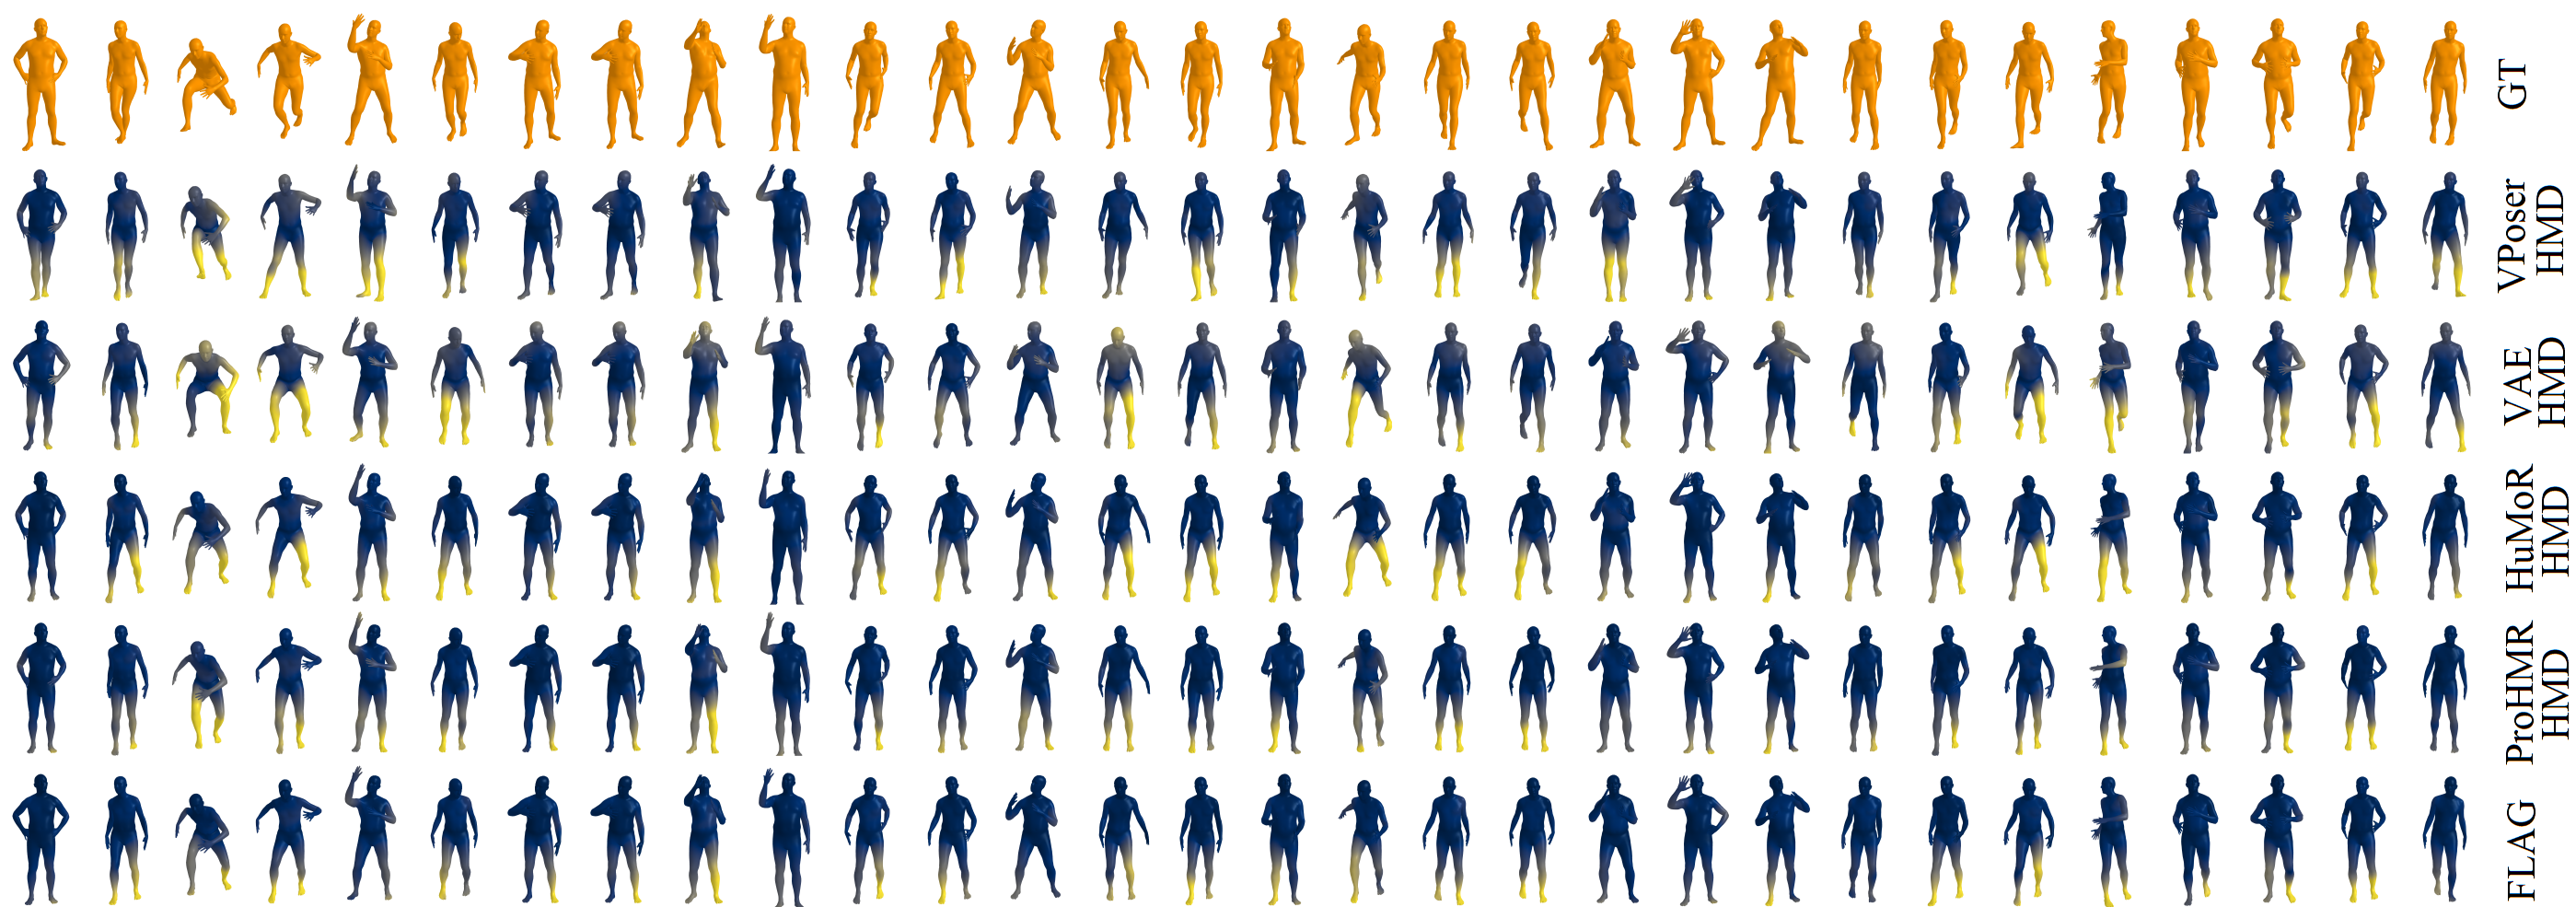}\\
         \includegraphics[width=\textwidth]{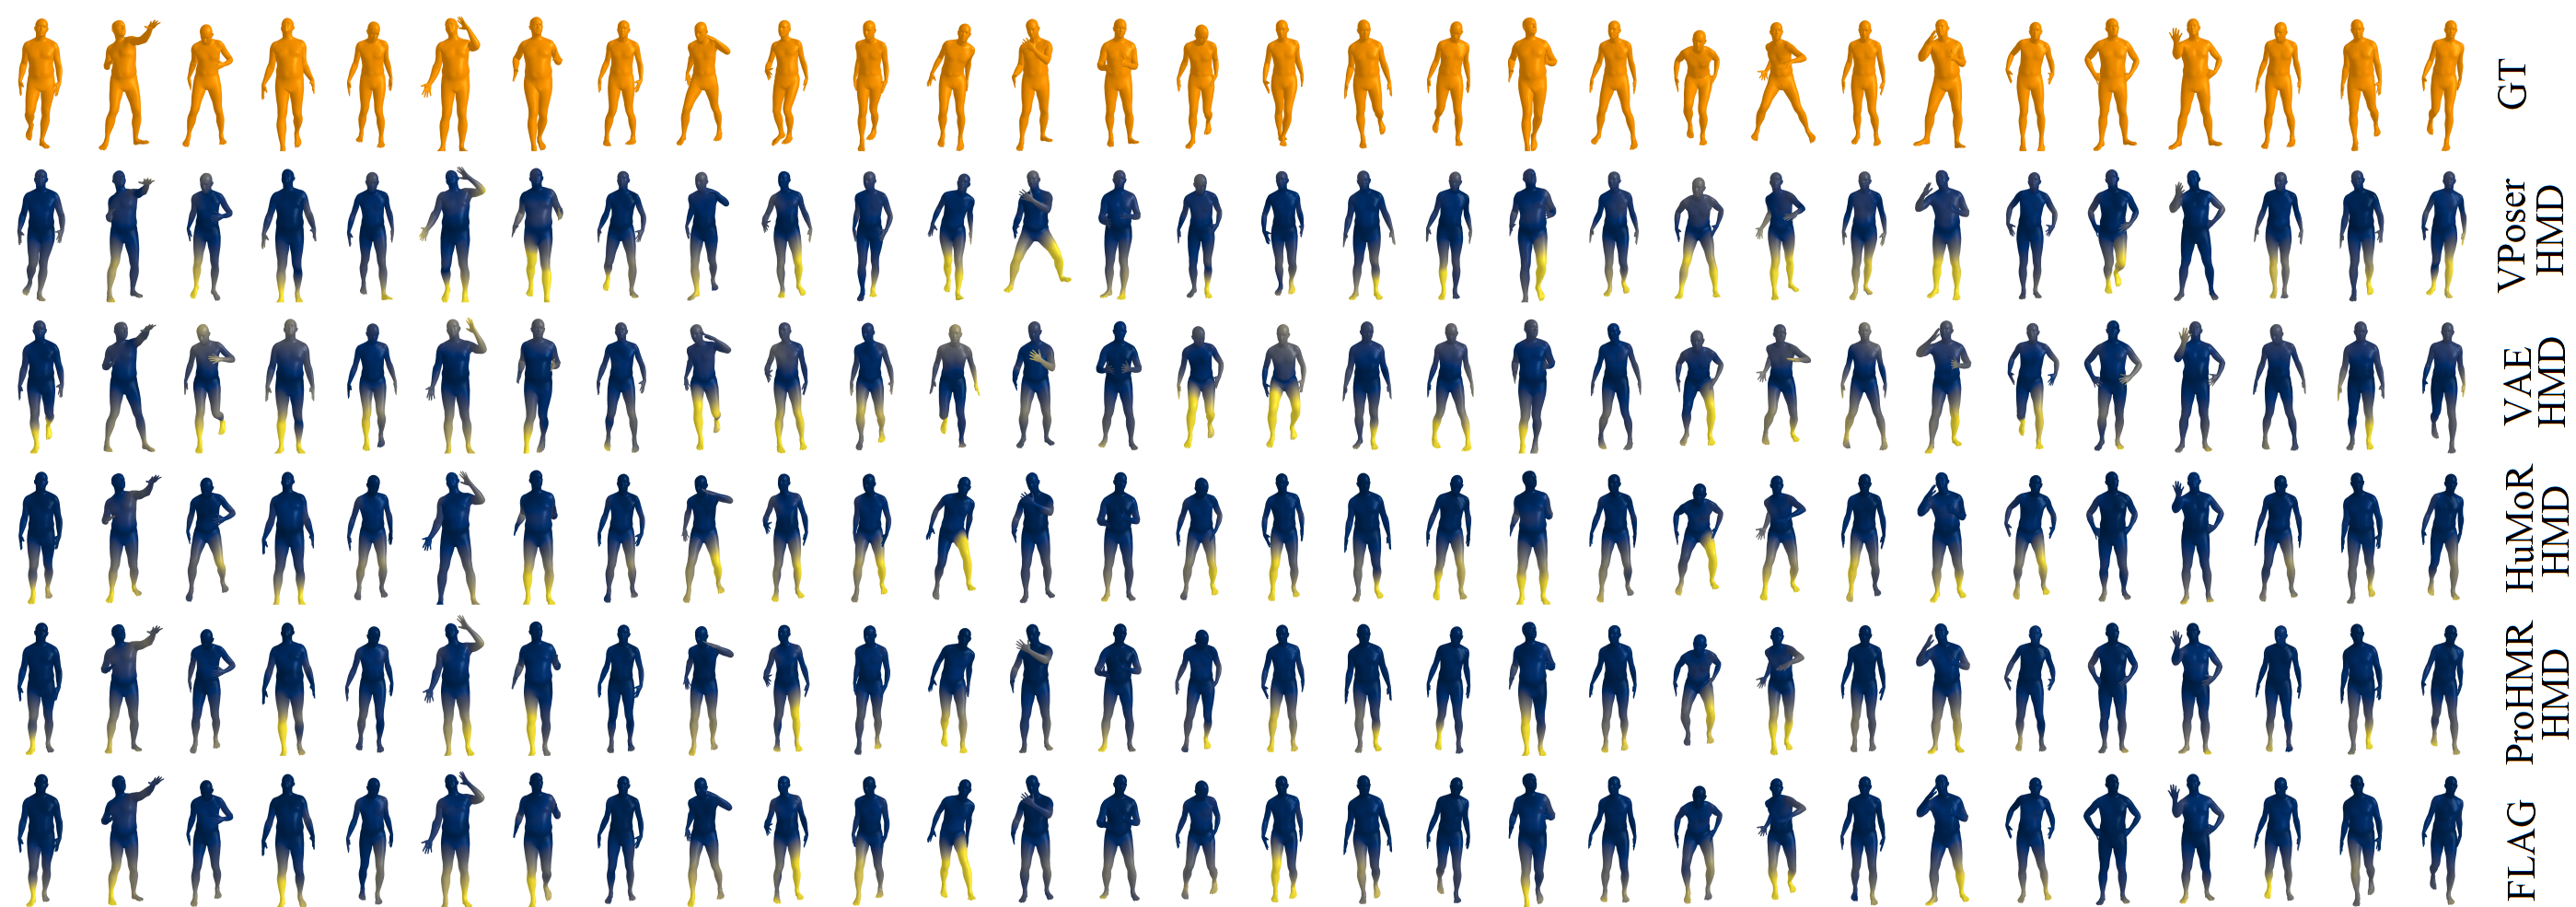}\\
         \includegraphics[width=\textwidth]{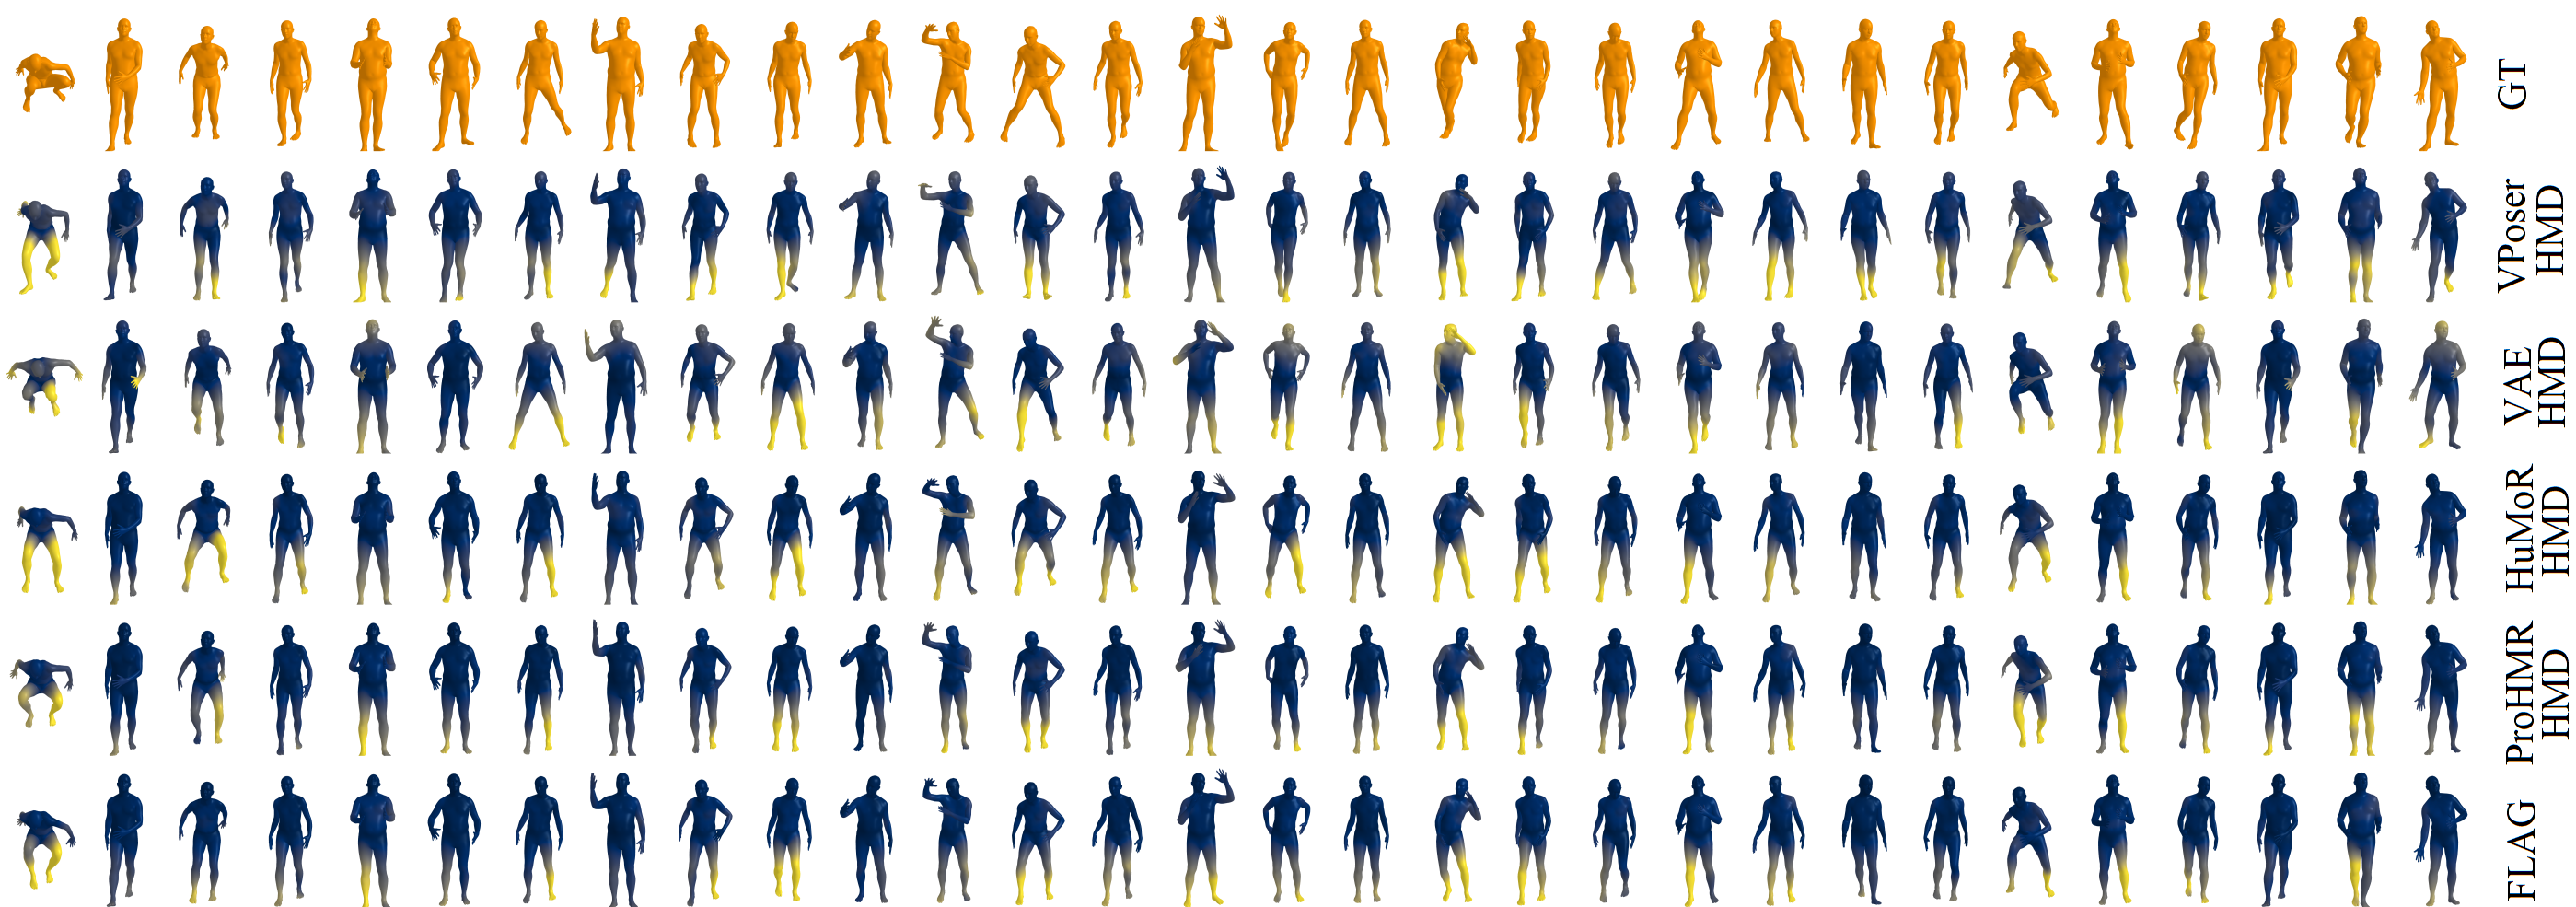}\\
    \end{tabular}
    
    \caption{Additional qualitative results. Best seen zoomed in. Note, in each segment of results, the last row represents our approach.}
    \label{fig:q1}
\end{figure*}

\begin{figure*}[!h]
    \centering
    \begin{tabular}{c}
         \includegraphics[width=\textwidth]{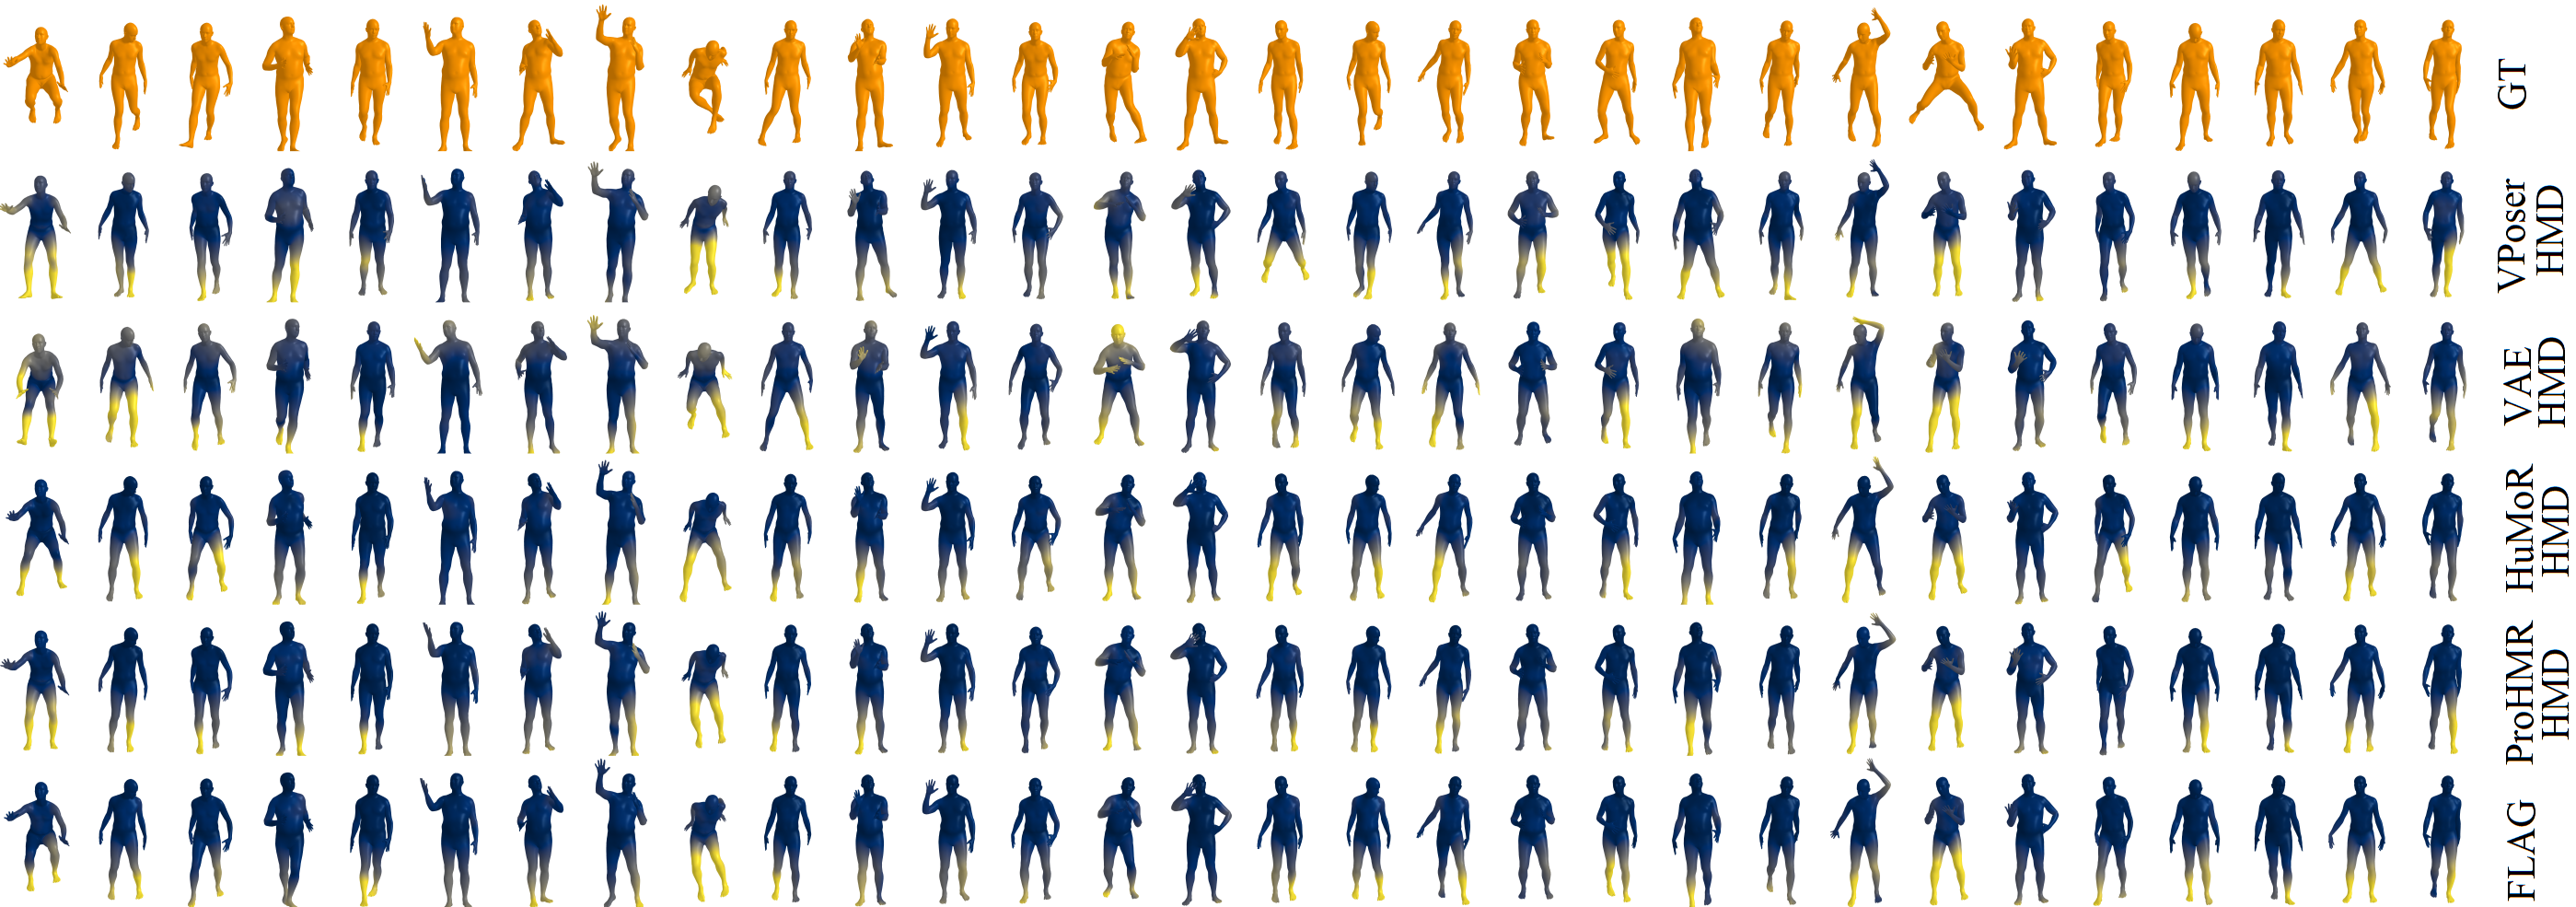}\\
         \includegraphics[width=\textwidth]{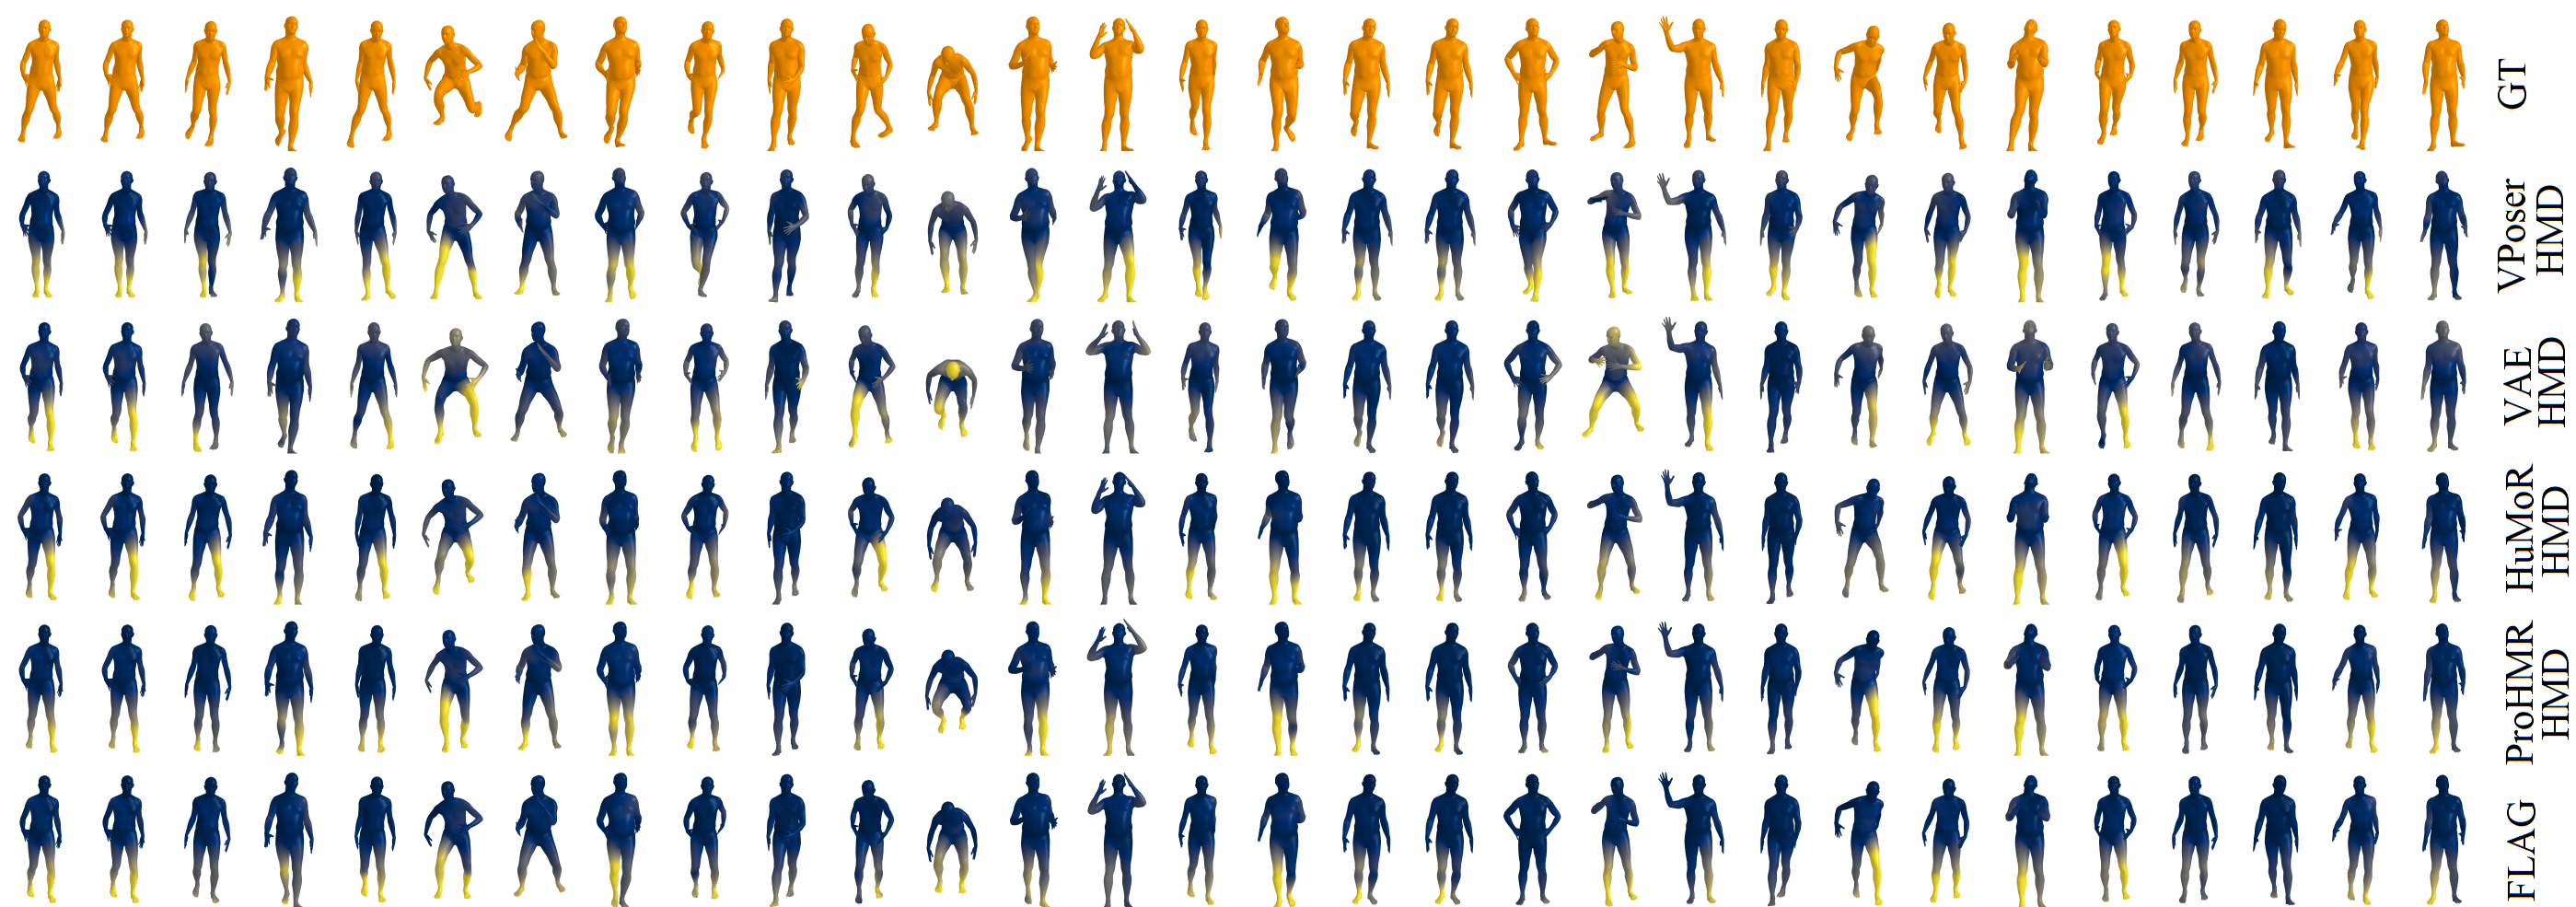}\\
         \includegraphics[width=\textwidth]{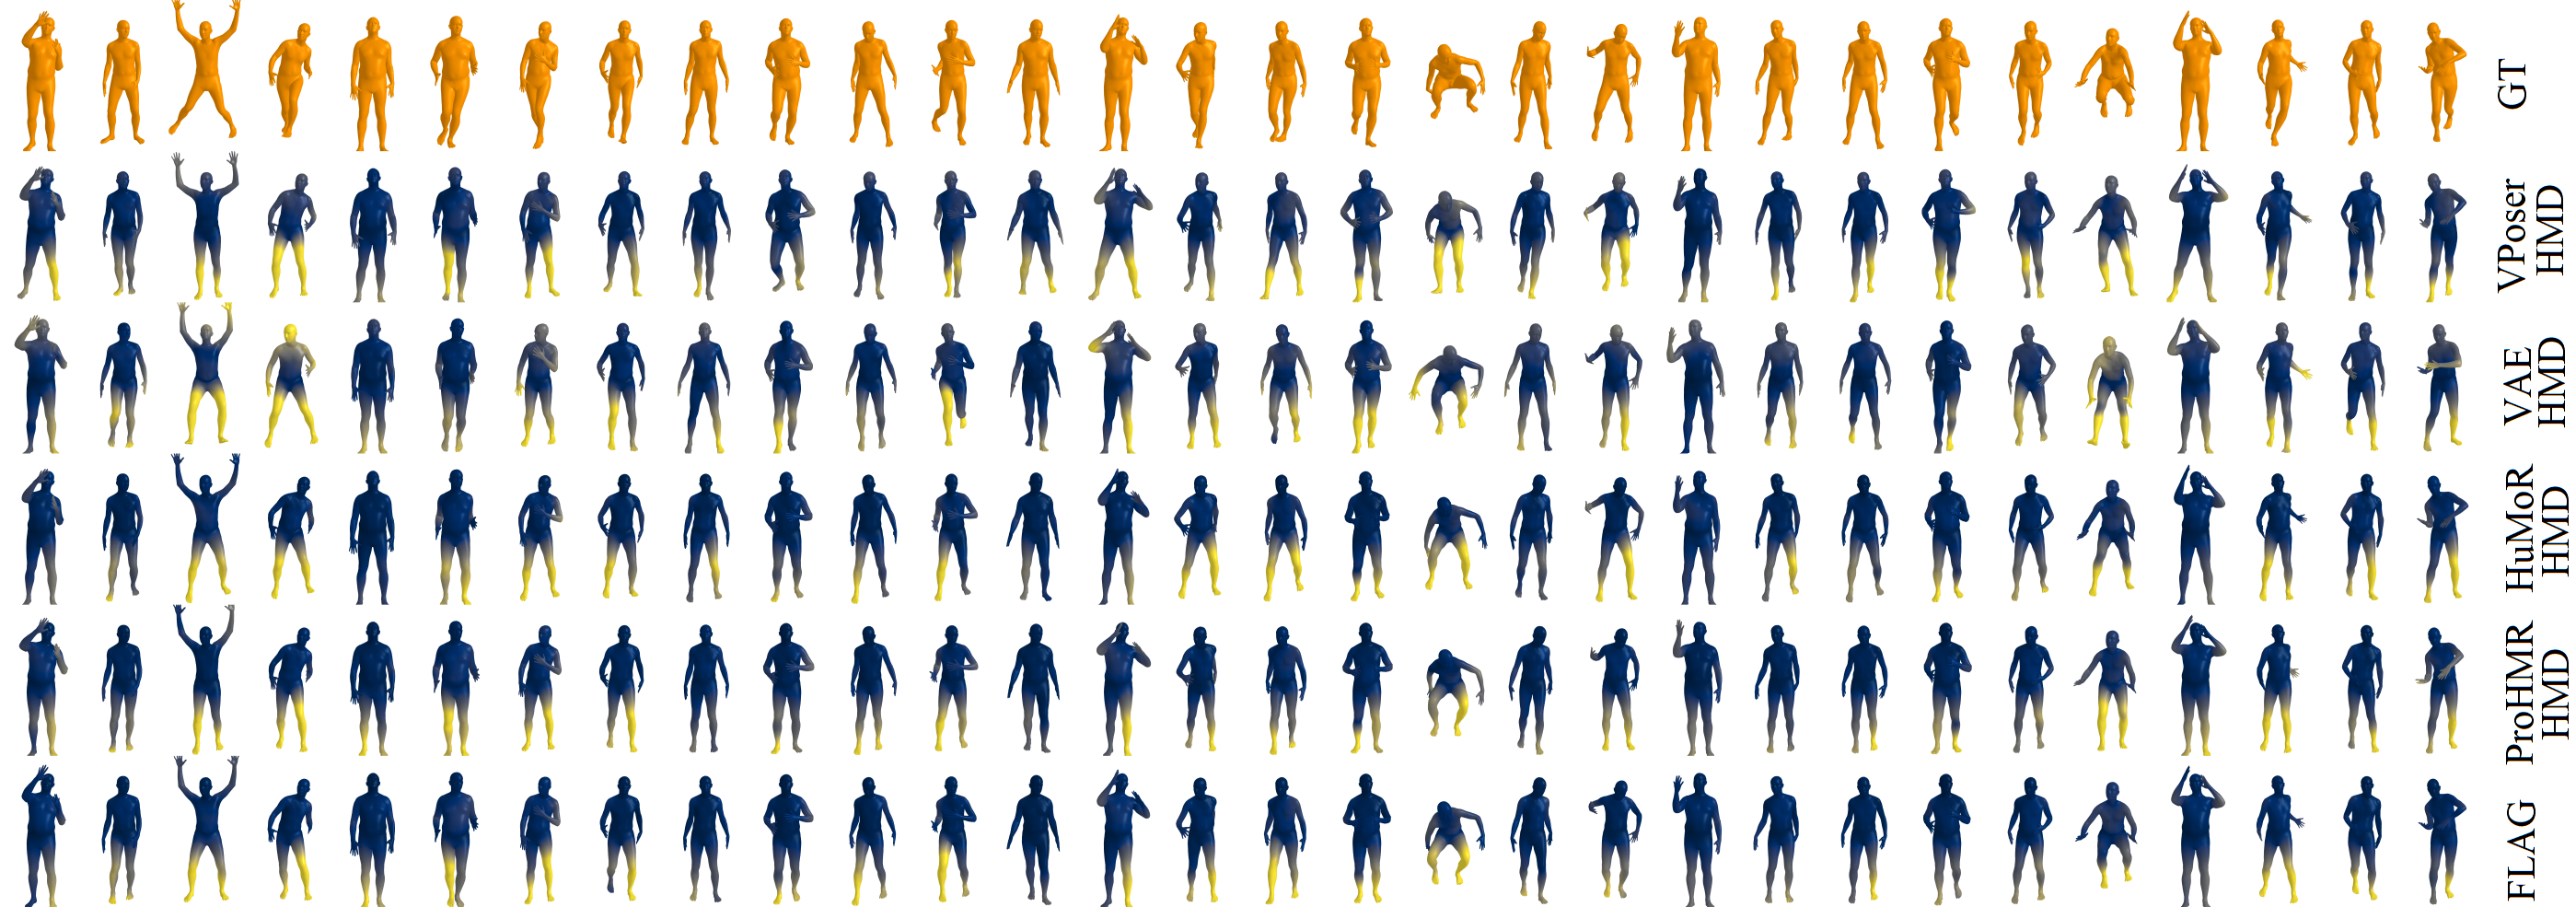}\\
    \end{tabular}
    
    \caption{Additional qualitative results. Best seen zoomed in. Note, in each segment of results, the last row represents our approach.}
    \label{fig:q2}
\end{figure*}

\begin{figure*}[!h]
    \centering
    \begin{tabular}{c}
         \includegraphics[width=\textwidth]{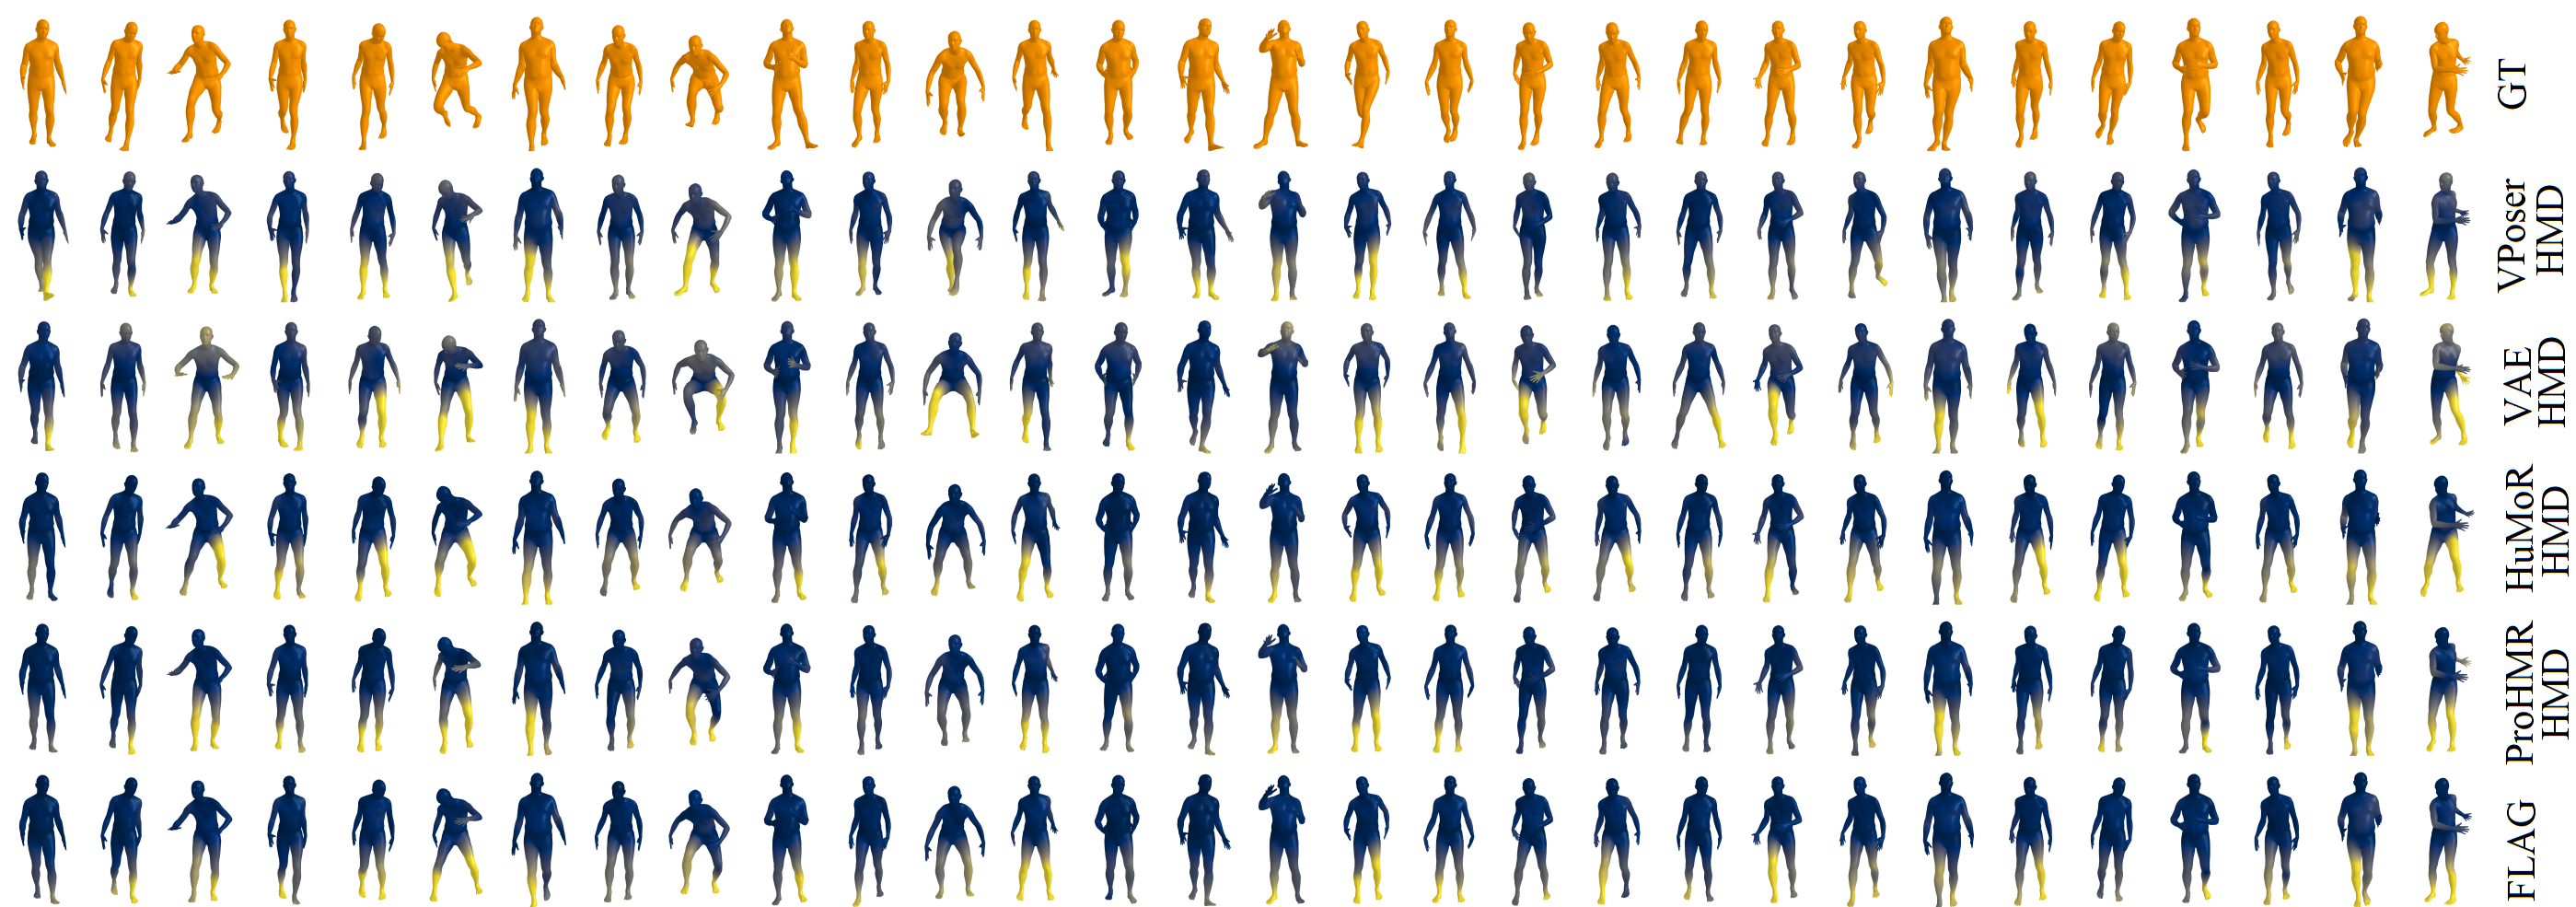}\\
         \includegraphics[width=\textwidth]{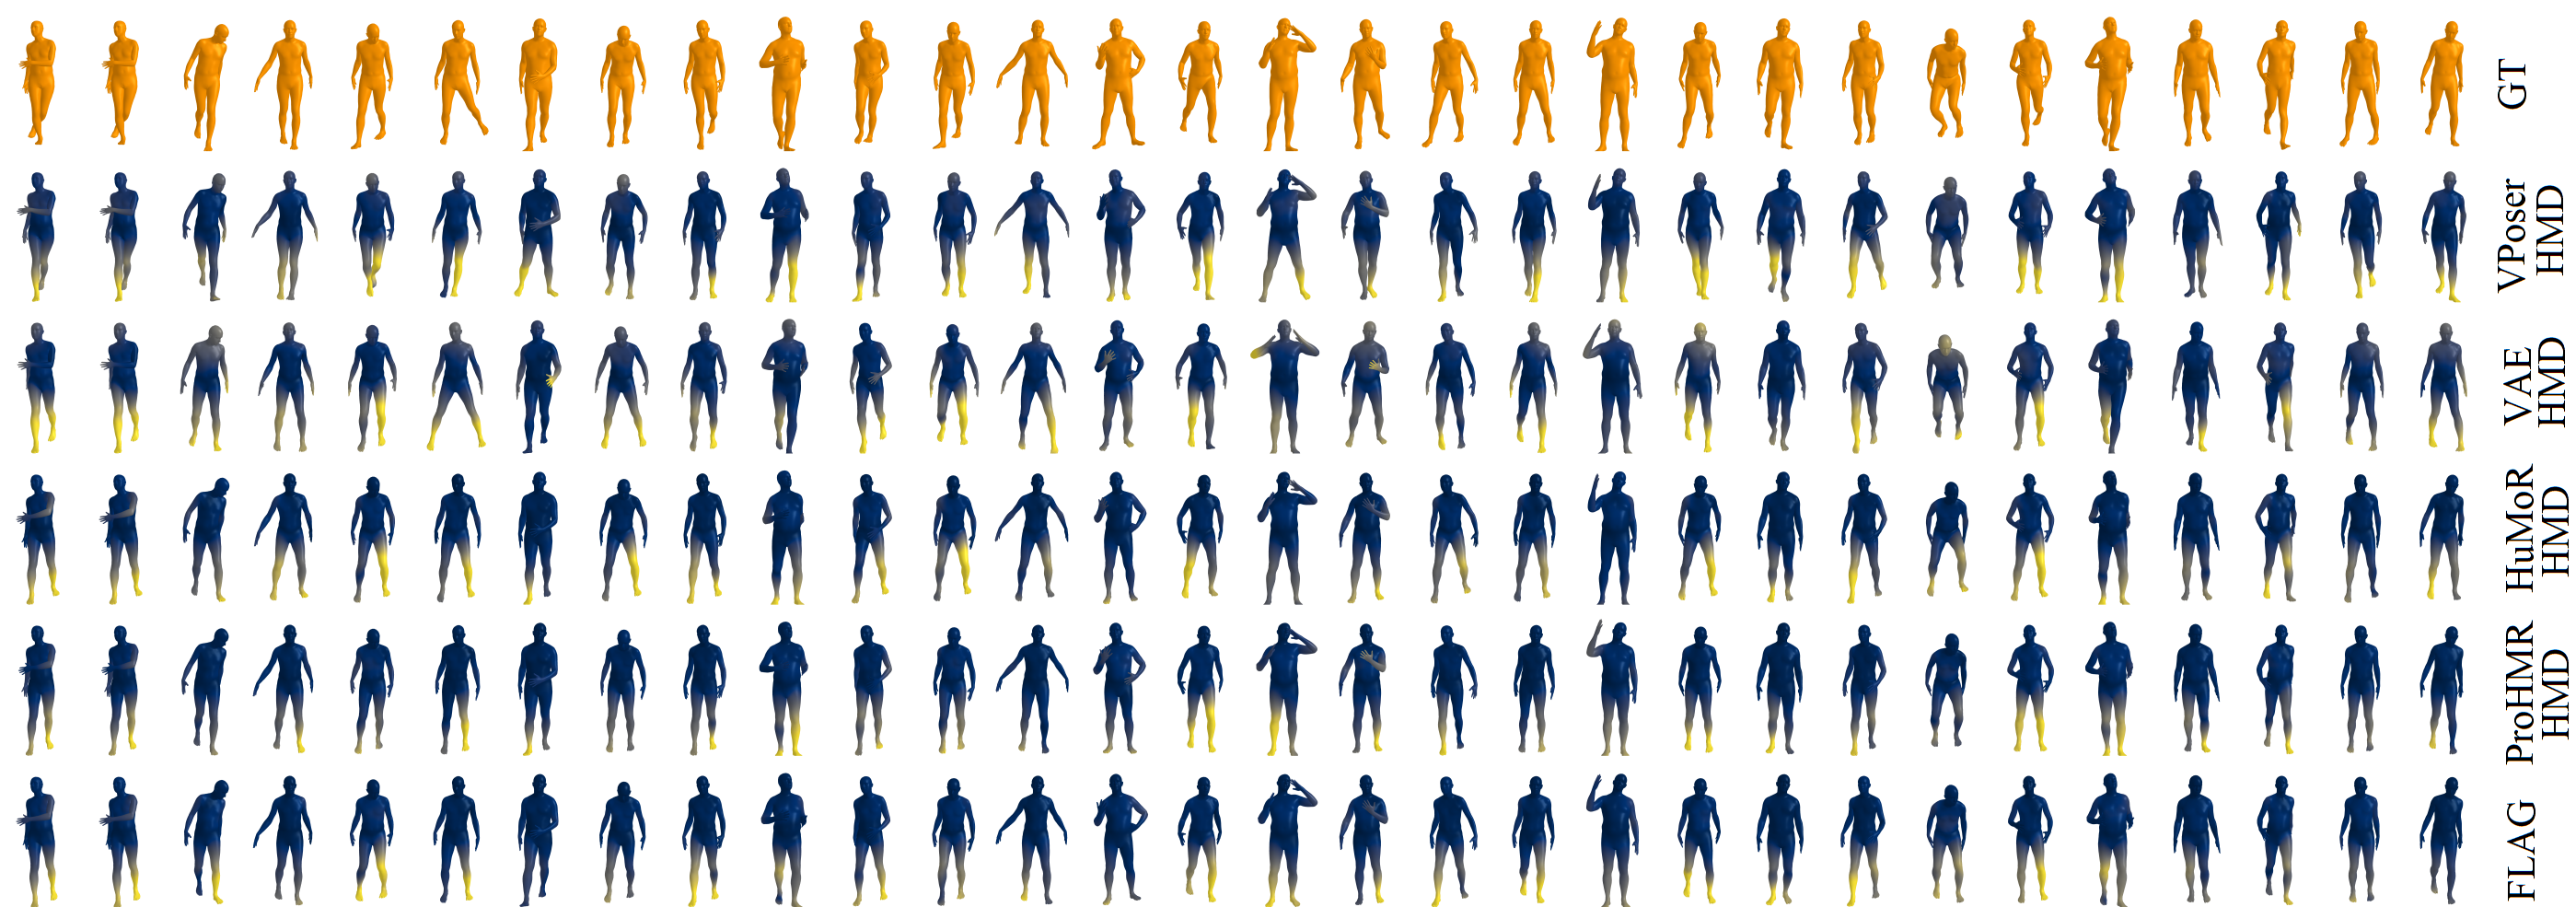}\\
         \includegraphics[width=\textwidth]{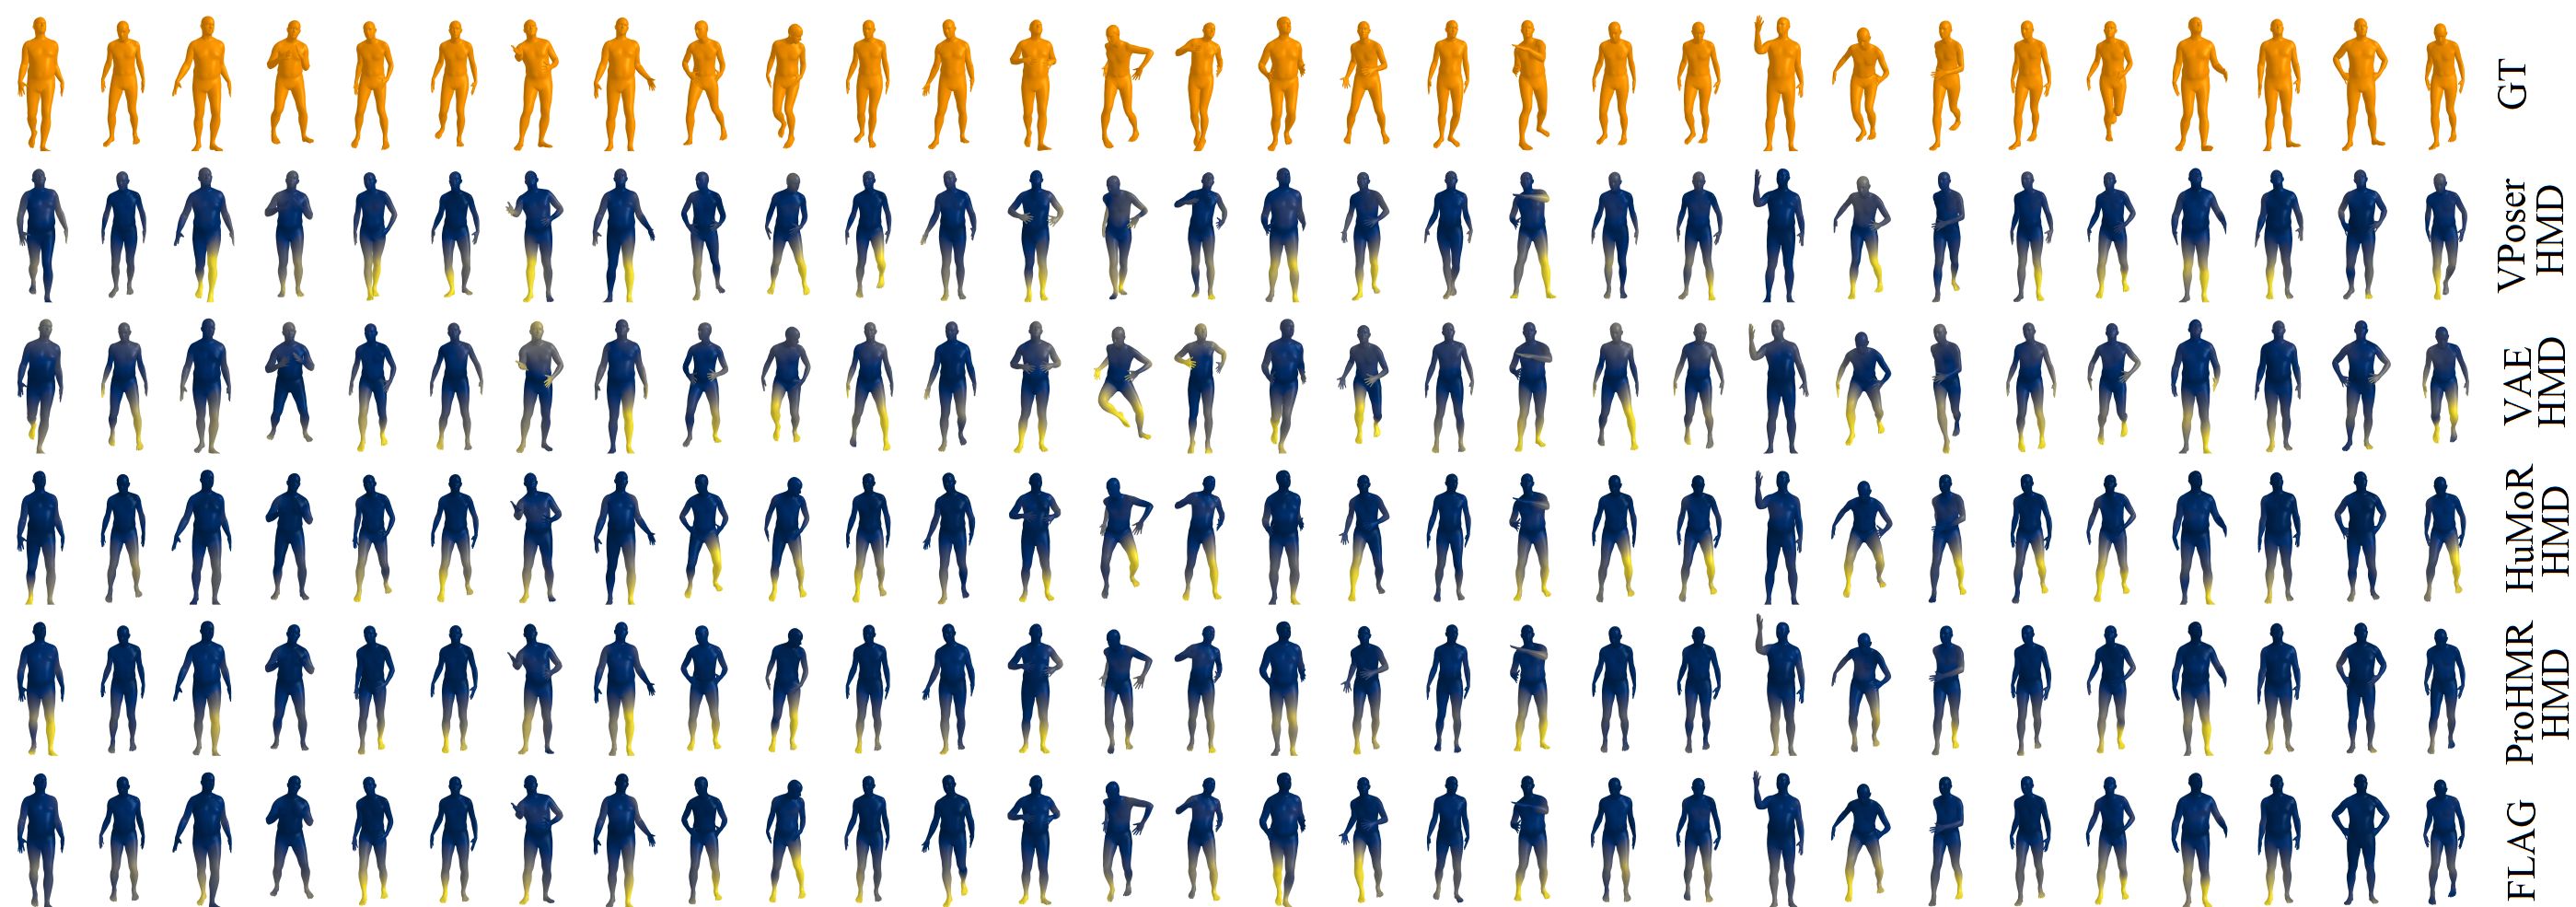}\\
    \end{tabular}
    
    \caption{Additional qualitative results. Best seen zoomed in. Note, in each segment of results, the last row represents our approach.}
    \label{fig:q3}
\end{figure*}

In this section, we provide additional qualitative results of our approach, as well as for all other baselines, in Fig.~\ref{fig:q1} to Fig.~\ref{fig:q3} shown in the next three pages. Note that the examples are not hand picked.
